# Supplementary material for: Low dephasing and robust micromagnet designs for silicon spin qubits
Source: arXiv:2108.10769 source file (2021-08-24)
Supplement: Supplementary file 1 [file Suppl_Info.pdf]

# Suppl. Infor. for Low Dephasing and Robust Micromagnet Designs for Silicon Spin Qubits

N. I. Dumoulin Stuyck[1,2], F. A. Mohiyaddin[2], R. Li[2], M. Heyns[1], B. Govoreanu[2] & I. P. Radu[2]

**Affiliations**
[1]Department of Materials Engineering (MTM), KU Leuven, B-3001 Leuven, Belgium
[2]imec, B-3001 Leuven, Belgium

### SI-1 Hamiltonian

We separate the total Hamiltonian of the system in a charge and spin part:

$$\widehat{\boldsymbol{H}} = \widehat{\boldsymbol{H}}_{\mathbf{charge}} + \widehat{\boldsymbol{H}}_{\mathbf{spin}}$$

with

$$\widehat{\boldsymbol{H}}_{\mathbf{charge}} = -\frac{\hbar^2}{2m_t}\left(\frac{d^2}{dx^2}+\frac{d^2}{dy^2}\right)-\frac{\hbar^2}{2m_l}\left(\frac{d^2}{dz^2}\right)+\frac{1}{2}m_t\left(\omega_x^2x^2+\omega_y^2y^2\right)-eF_zz+U_0\Theta\left(z-z_I\right)+eV_{\text{noise}}(x,y,z)+eV_{\text{drive}}(x,y,z)$$

$$\widehat{\boldsymbol{H}}_{\mathbf{spin}} = g\mu_B\mathbf{B}\cdot\boldsymbol{\sigma} + g\mu_B(\mathbf{r_n}\cdot\boldsymbol{\nabla})(\mathbf{B}\cdot\boldsymbol{\sigma}) + g\mu_B(\mathbf{r_d}\cdot\boldsymbol{\nabla})(\mathbf{B}\cdot\boldsymbol{\sigma}).$$

Here, $m_{t,l}$ are the electron's transverse and longitudinal effective masses, $\omega_i$ the harmonic confinement potential frequency along $i^{\text{th}}$ direction, $F_Z$ the electric field along the z direction, $U_0\Theta(z - z_I)$ the step-potential at the interface $z_I$ with barrier height $U_0$, and $V_{\text{noise}}$ and $V_{\text{drive}}$ the noise and driving potential, respectively.
For $\widehat{\boldsymbol{H}}_{\mathbf{spin}}$: $\mathbf{B} = B_x\widehat{\boldsymbol{x}} + B_y\widehat{\boldsymbol{y}} + B_z\widehat{\boldsymbol{z}}$ is the external magnetic field vector, $\boldsymbol{\sigma} = \sigma_x\widehat{\boldsymbol{x}} + \sigma_y\widehat{\boldsymbol{y}} + \sigma_z\widehat{\boldsymbol{z}}$, and $\mathbf{r_n}$ and $\mathbf{r_d}$ the electron wavefunction displacement vectors due to noise and driving electric fields, respectively. $\hat{x}$, $\hat{y}$ and $\hat{z}$ are unit vectors along the three Cartesian axes, and $\sigma_x$, $\sigma_y$ and $\sigma_z$ are Pauli spin smatrices.

We assume the displacement in the z-direction to be very small compared to the x- and y-direction due to the strong vertical confinement at the interface. Further, we assume an external applied magnetic field along the y-direction such that $\boldsymbol{B} = B_0\widehat{\boldsymbol{y}}$. Magnetic field gradients ($dB_y/d_x$ and $dB_y/d_y$) along the y-direction contribute to spin dephasing, while perpendicular gradients ($dB_x/d_y$ and $dB_z/d_y$) enable spin manipulation. This allows us to restrict our analysis to the gradients mentioned in the main text.

### SI-2 Charge noise PSD amplitude

An electrostatic confinement energy for electrons in Silicon quantum dots of 1 meV is assumed, and is consistent with results presented in Ref. 1. Directionality of the electric field noise in the dephasing (y) direction is compensated with a pre-factor equal to $\sqrt{2}$. From the electric field, the r.m.s. charge noise Power Spectral Density (PSD) amplitude $\sigma_{cn}$ is calculated assuming a commonly reported 1/f noise spectral density and a dot-to-trap distance $l_0$ of 70 nm, based on the typical distance between gate interface and quantum dot in SiGe devices[2,3]:

$$\sigma_{cn} = \frac{el_0}{\sqrt{ln(\frac{f_1}{f_0})}}.$$

Here, $e$ is the electron charge, and $f_0$ and $f_1$ are the low and high frequency limit which we take based on the spin relaxation time and dephasing rate as 1 Hz and 10 kHz, respectively[1].

## SI-3 Supplementary Figures

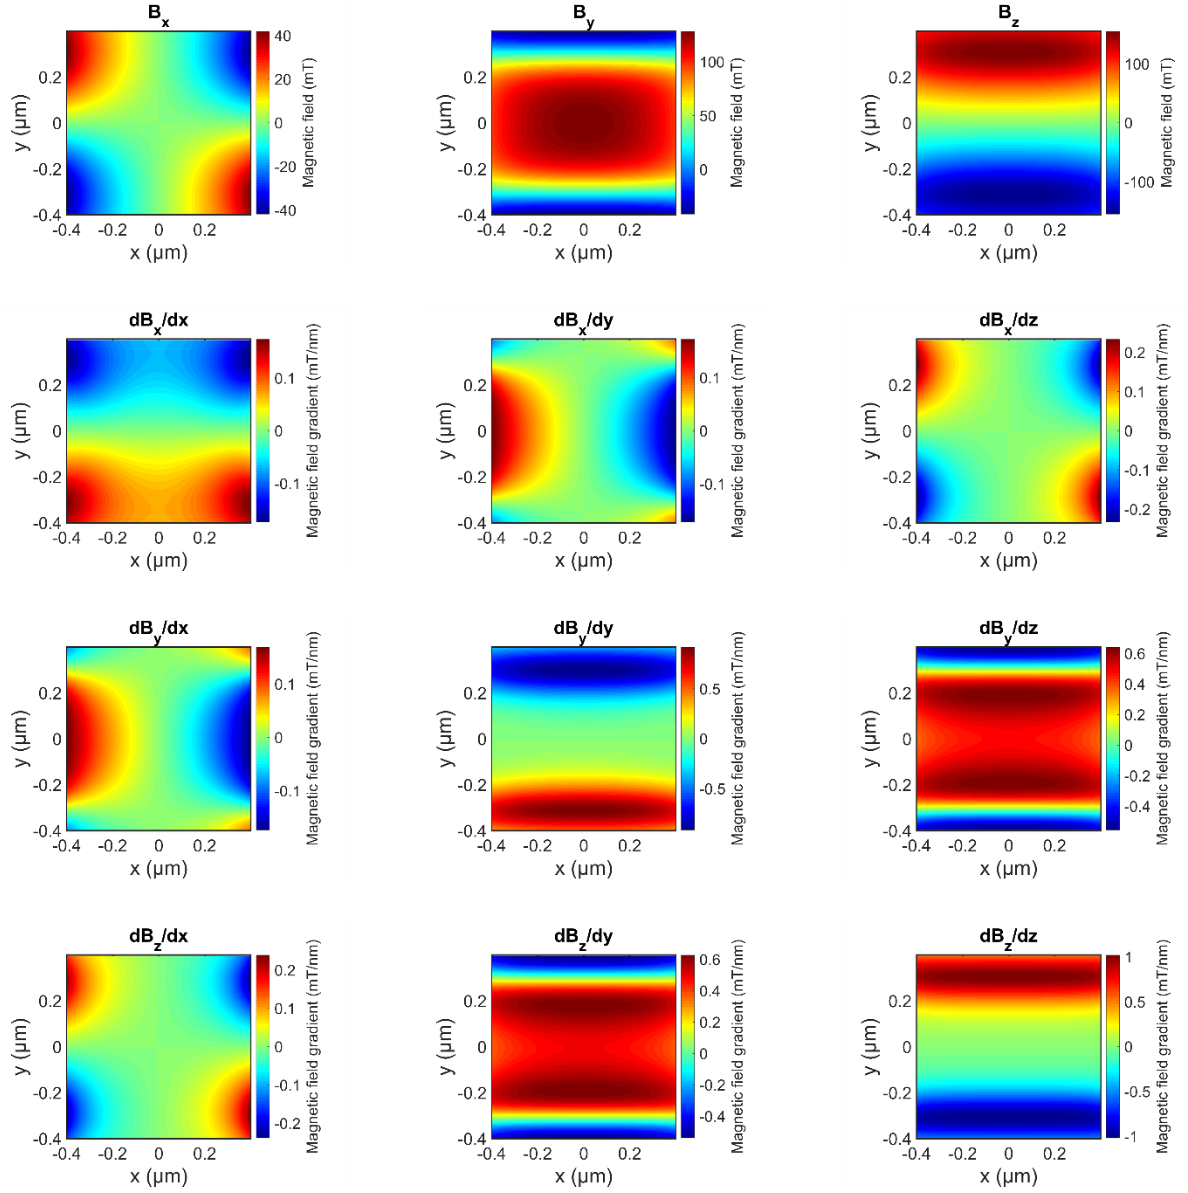


**SFIG.1** Magnetic field and field gradient matrix for the micromagnet with a 600 nm gap size, taken at $d_{QDM} = 150$ nm.

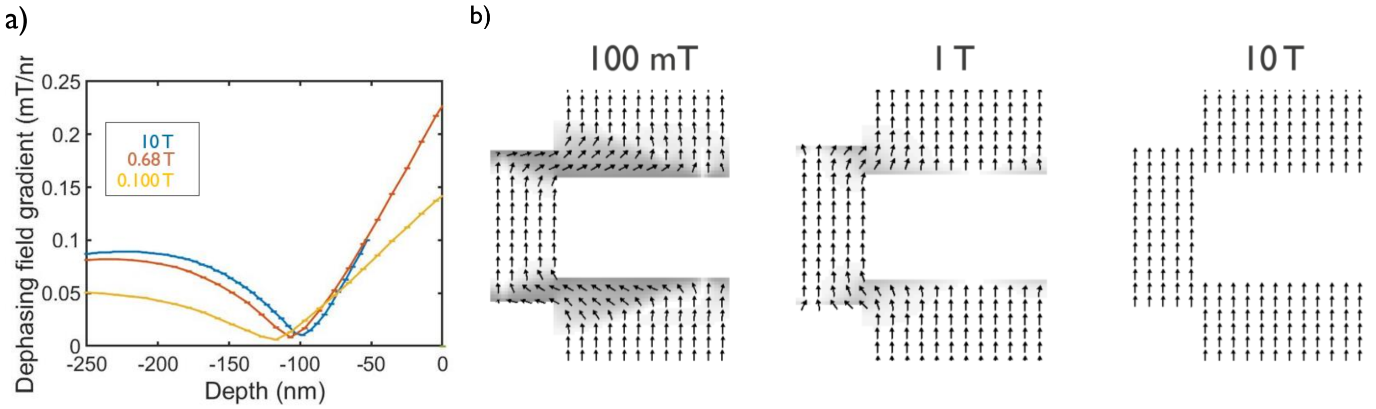


**SFIG.2** Influence of the magnetizing field on the optimal $d_{QDM}$. By lowering the external applied field, less of the micromagnet volume is magnetized. a) Dephasing field gradient as a function of depth for different external applied fields. Optimized dot-magnet separation changes by ~ 20%, for changes in magnetizing field from 10T to 100 mT. b) Total magnetization (arrows) and magnetization vector y-component (shading) for different external magnetic fields (indicated above) taken at the magnet center.

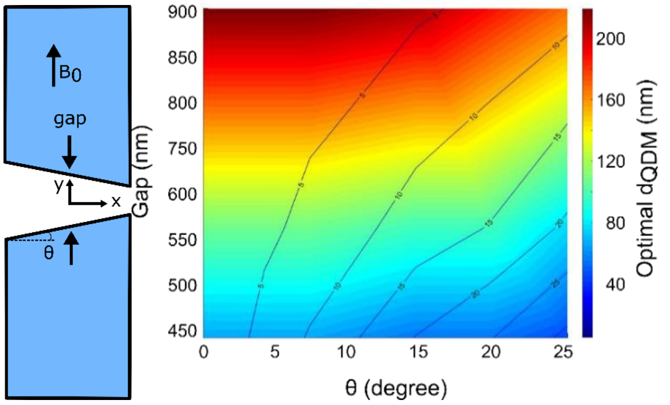


**SFIG. 3** Optimal $d_{QDM}$ for a different design that enables qubit addressability and manipulation, which we call the V-shape design (shown on the left) as a function of its two design parameters, gap and angle. The contour lines denote $\Delta B_Z$ (in mT) at x = y = 0 µm. For each desired $\Delta B_Z$ the micromagnet architecture can be optimized either by fabrication ($d_{QDM}$) or design (gap and/or angle).

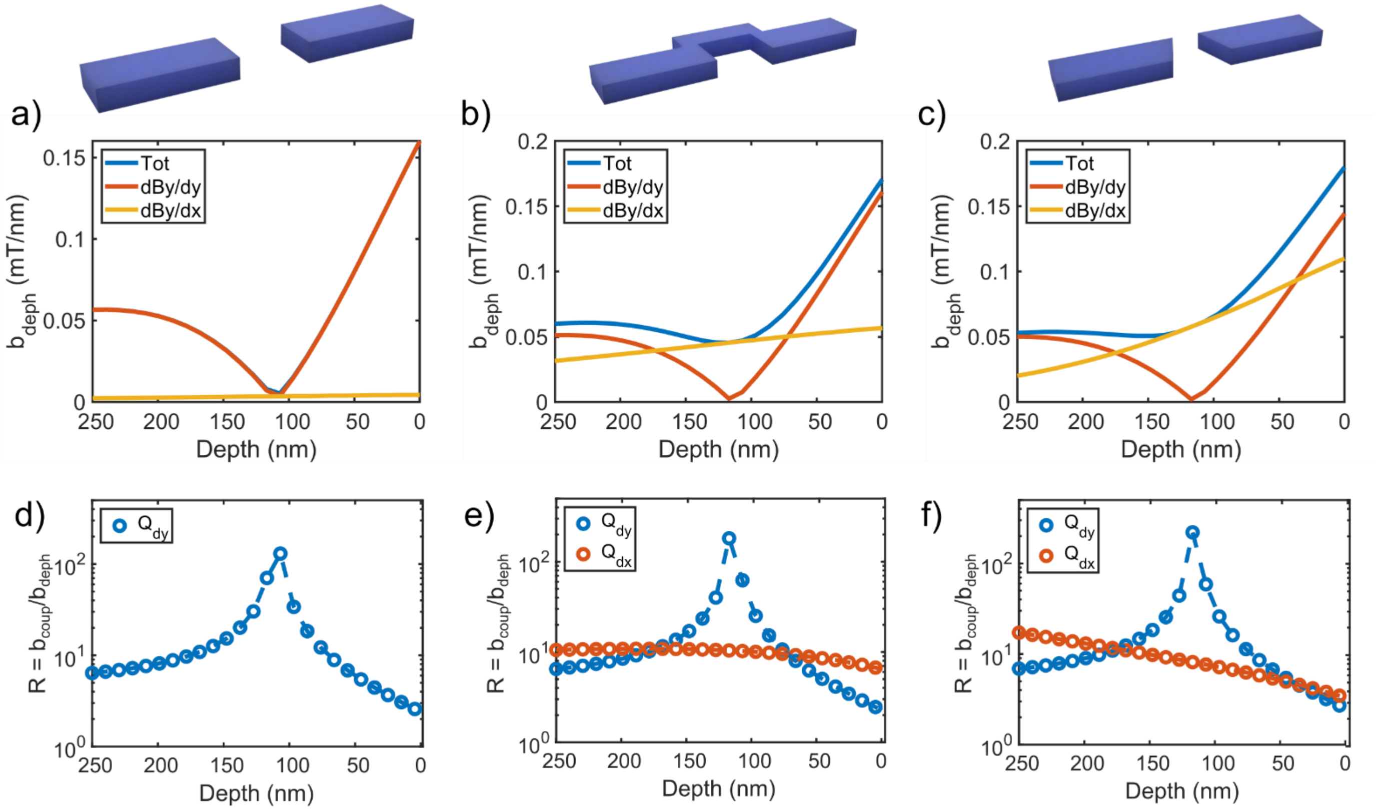


**SFIG. 4** a)-c) Dephasing gradients along $dB_y/d_y$ (red), $dB_y/d_x$ (yellow) and $tot \equiv \sqrt{(dBy/dy)^2 + (dBy/dx)^2}$ for three different designs shown above the plots. All topologies have a 600 nm central gap and gradients are taken at x = y = 0 µm. Design shown in a) is used for single qubit experiments including spin-to-photon coupling architectures[4,5]. We attribute the non-zero $dB_y/d_x$ gradient due to simulation grid size and partial magnetization. Designs shown in b) and c) offer qubit addressability at the cost of a finite dephasing gradient along x at the optimal depth. d)-f) *R*, defined as $b_{coup}/b_{deph}$ for dephasing gradients along dy (blue) and dx (red).

## Supplementary References


1 J. Yoneda, K. Takeda, T. Otsuka, T. Nakajima, M.R. Delbecq, G. Allison, T. Honda, T. Kodera, S. Oda, Y. Hoshi, N. Usami, K.M. Itoh, and S. Tarucha, Nat. Nanotechnol. 13, 102 (2018).

2 P. Huang and X. Hu, Phys. Rev. B 89, 195302 (2014).

3 A. Noiri, K. Takeda, J. Yoneda, T. Nakajima, T. Kodera, and S. Tarucha, Nano Lett. 20, 947 (2020).

4 X. Mi, J. V. Cady, D. M. Zajac, P. W. Deelman, and J. R. Petta, "Strong coupling of a single electron in silicon to a microwave photon," Science 355, 156–158 (2017).

5 N. Samkharadze, G. Zheng, N. Kalhor, D. Brousse, A. Sammak, U. C. Mendes, A. Blais, G. Scappucci, and L. M. Vandersypen, "Strong spin photon coupling in silicon," Science 359, 1123–1127 (2018)
